# Supplementary material for: SkillAdaptor: Self-Adapting Skills for LLM Agents from Trajectories
Source: arXiv:2606.01311 source file (2026-05-31)
Supplement: Supplementary file 2 [file experiments_ablation.tex]

% Ablation prose and table moved to body/ablation_main.tex (main text).
% Full ablation section preserved for reference in appendix/experiments.tex.
\input{tables/claw_round_scores}
